# Supplementary material for: Risk Set Matched Difference-in-Differences for the Analysis of Effect Modification in an Observational Study on the Impact of Gun Violence on Health Outcomes
Source: arXiv:2305.04143 source file (2024-05-31)
Supplement: Supplementary file 1 [file matchDID_supp_sec1.tex]

\subsection{Details on Risk Set Matching}
Risk set matching \citep{LiYunfeiPaul2001BRSM} matches each newly treated unit at time $t$ with controls who are not yet treated based on covariate information up to time $t$. 
Once a control is used in a match, it is discarded from the pool of potential controls for future-treated units.
This structure enables the use of traditional methods for randomization and sensitivity analysis, as in \cite{RN55} via the following model for the hazards of treatment at time $t$ for unit $i$:
\begin{align}
\label{eq_hazards}
h_{tij} = \lim_{\delta \to 0} \mathbb{P}\left(t + \delta \geq Z_{ij} \geq t | Z_{ij} \geq t\right) / \delta = \exp\left(\xi\left(\bm{x}_{tij}(\infty)\right) + \gamma u_{tij} \right)
\end{align}
where $u_{tij}$ is an unmeasured variable, $\xi(\cdot)$ is an arbitrary function, and $\gamma \in \mathbb{R}$.
Thus, the hazards of treatment at time $t$ is a function of the control potential covariates (which, by Assumption 2, are observed because the units are not yet treated) and unmeasured confounders, where these two sets of variables do not interact.
When $\gamma = 0$, there is no unmeasured confounding (i.e., as in Assumption 4), this places no restrictions on the relationship between the potential covariates and the hazards.
The no-interaction relationship between the unmeasured variables and the other covariates enables the use of conventional sensitivity analyses for unmeasured confounding \citep{RN6}.

Under \eqref{eq_hazards}, we have:
\begin{align}
\label{eq_assignment}
\mathbb{P}\left(\bm{W} = \bm{w} | \mathcal{D} \right) = \prod_{i = 1}^{I} \dfrac{\exp\left(\gamma \sum_{j=1}^{n_i} w_{ij} u_{ij}\right)}{\sum_{j=1}^{n_i} \exp \left(\gamma u_{ij}\right)}
\end{align}
where $\bm{W} = (W_{11}, ..., W_{1n_1}, ..., W_{In_I})$ and $\mathcal{D}$ denotes the matching design (i.e., the matched sets).
